# Supplementary material for: Nezha: Deployable and High-Performance Consensus Using Synchronized Clocks
Source: arXiv:2206.03285 source file (2023-03-24)
Supplement: Supplementary file 2 [file supplementary.tex]

\section{Supplementary Experiment Results}
\label{sec-supplement}

\begin{figure}[!htbp]
  \centering
  \begin{minipage}{1\linewidth}
    \centering
    \subcaptionbox{Closed-loop\label{fig-closed-scalability}}
      {\includegraphics[width=0.8\linewidth]{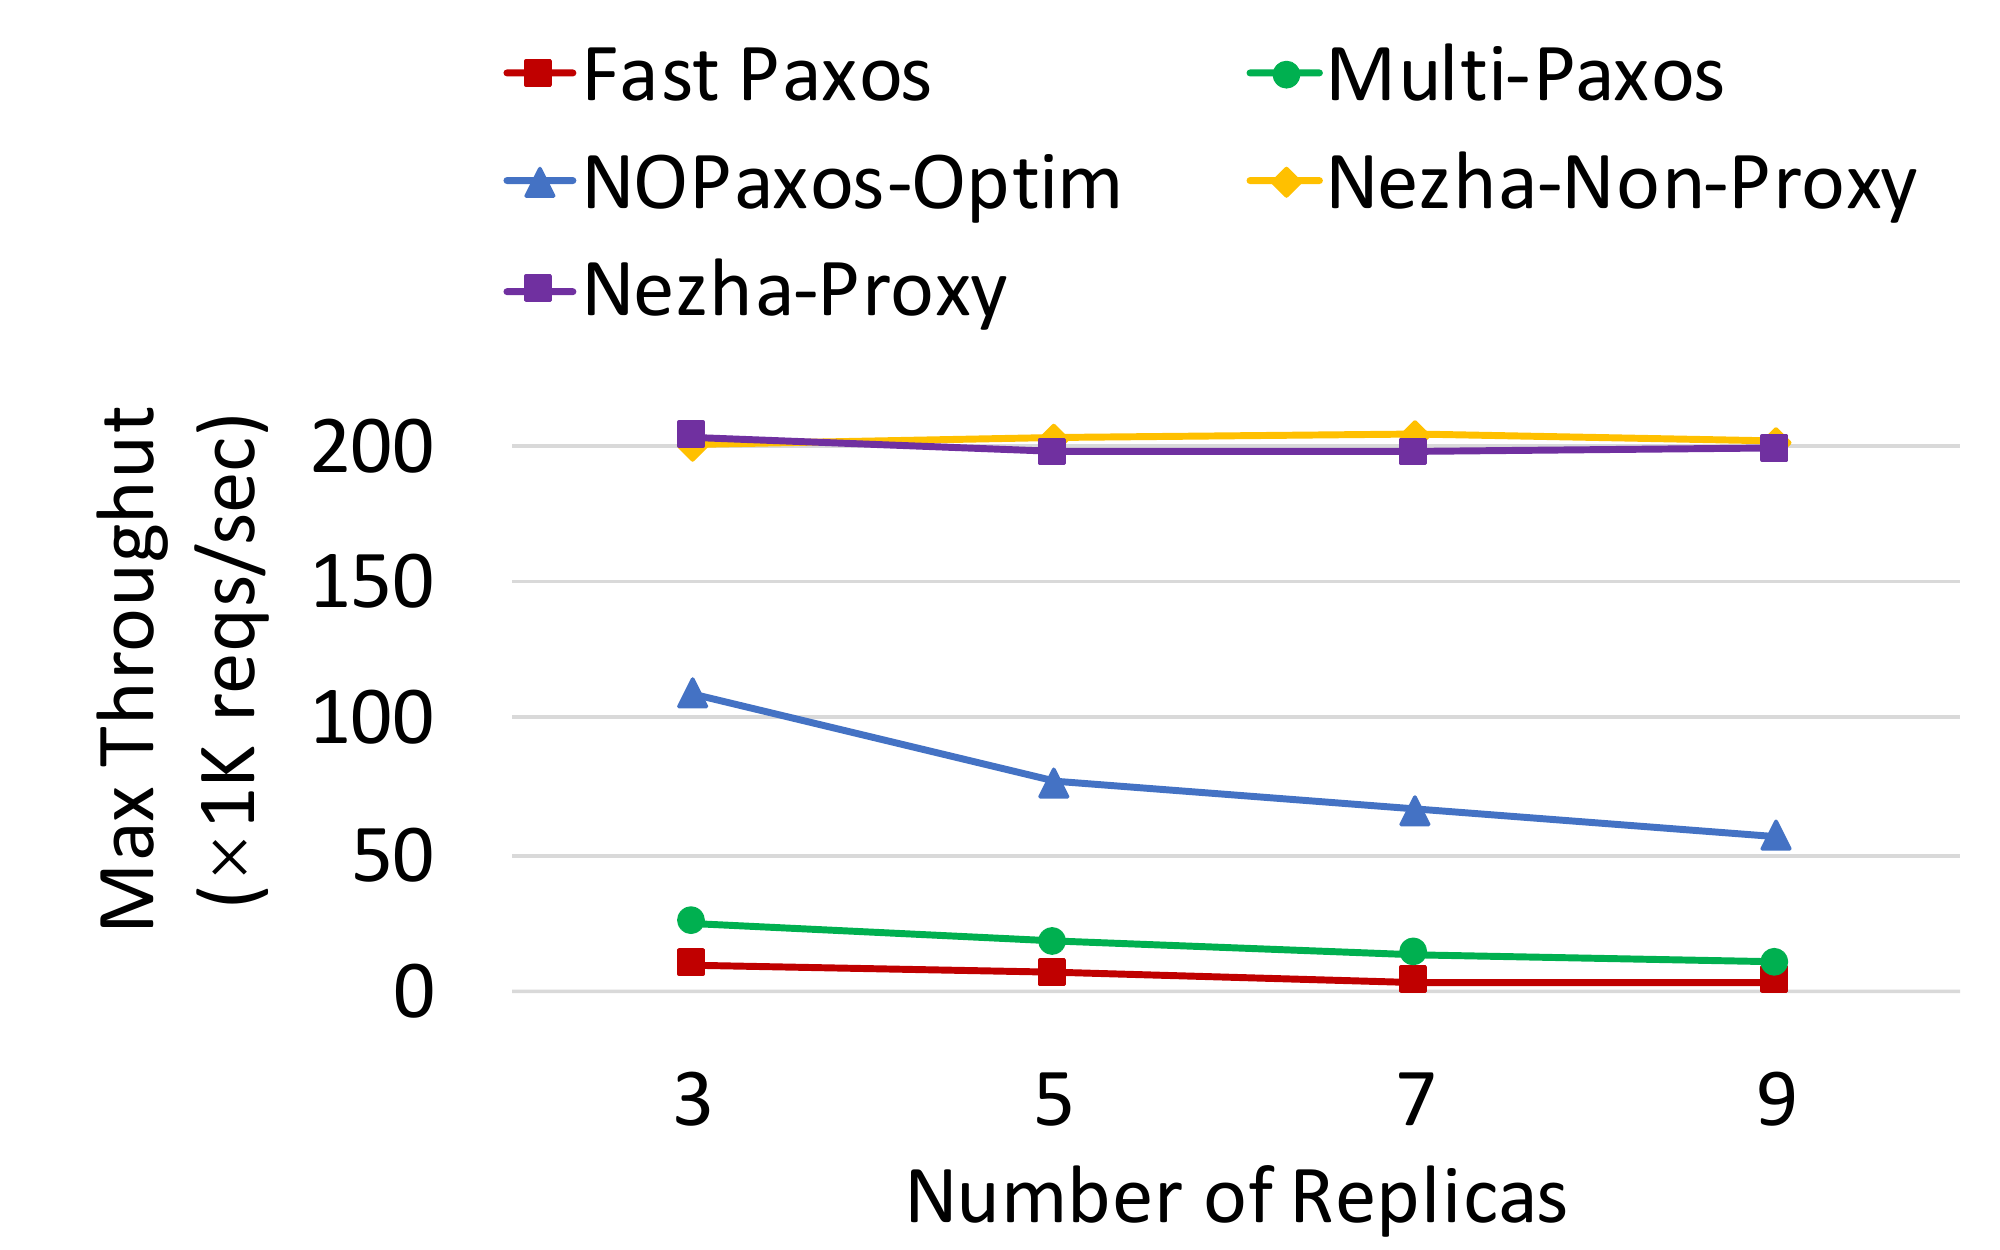}}
    \subcaptionbox{Open-loop\label{fig-open-scalability}}
      {\includegraphics[width=0.8\linewidth]{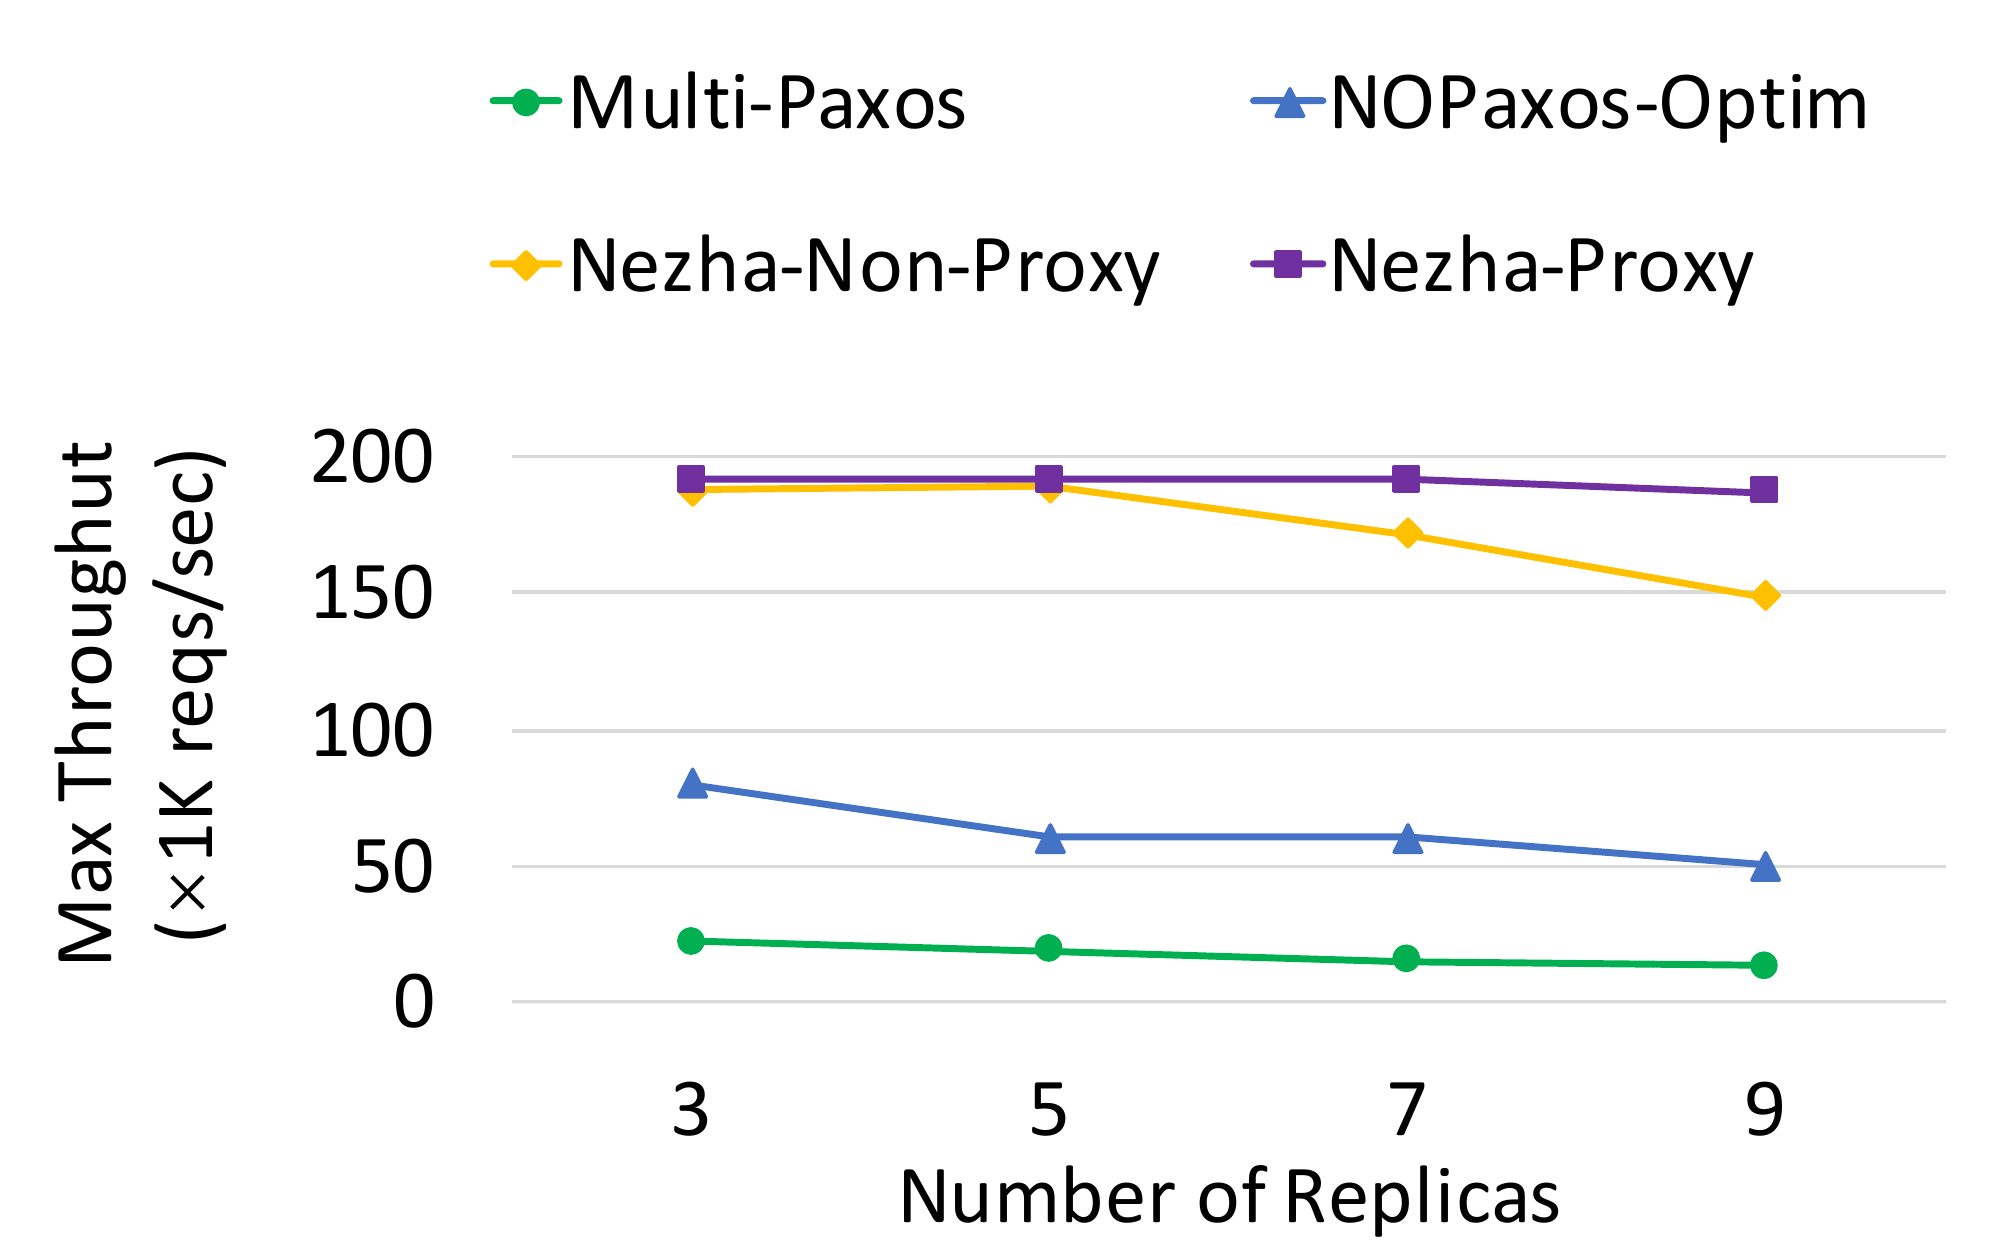}}
    \caption{Max throughput vs. number of replicas}
    \label{throughput-scalability}
  \end{minipage}
\end{figure}

Due to space limit, we have omitted some evaluation figures in the main text. We append these figures as below.

Figure~\ref{throughput-scalability} presents the scalability of throughput for \sysname and the three baselines. We omit the figure of closed-loop test (Figure~\ref{fig-closed-scalability}) in the main text. 

We can see that, both \sysname-Proxy and \sysname-Non-Proxy greatly outperform the baselines in both closed-loop and open-loop tests. In closed-loop tests, both \sysname-Proxy and \sysname-Non-Proxy maintain a high throughput, which is contributed by 150 clients, and each client only submit at a low rate ($\sim$1.3K reqs/sec). However, when it comes to open-loop tests with only 10 clients, \sysname-Non-Proxy suffers from serious degradation, because it requires the clients to multicast requests at high rates and conduct heavy quorum check, without proxies. By contrast, when equipped with proxies, neither replicas nor clients become bottlenecks, and the throughput of \sysname-Proxy remains high regardless of the number of replicas.

% \rv{Figures~\ref{throughput-scalability} demonstrates that \sysname has much higher throughput than the baselines under different number of replicas. \sysname without proxies suffer from little degradation in closed-loop tests, because the throughput is contributed by 150 clients and each client only submits at a low rate ($\sim$1.3K reqs/sec). However, in open-loop tests with only 10 clients, the throughput of \sysname without proxies distinctly degrades from 187.8K reqs/sec to 148.7K req/sec, as the number of replicas grows. This indicates that the clients become the new bottleneck when submitting at high rates. By contrast, when equipped with proxies, neither replicas nor clients become bottlenecks, and the throughput remains high regardless of the number of replicas. We further evaluate the proxy design in \S\ref{sec:proxy}.}  

Figure~\ref{proxy-eval-supplement} presents the effect of proxies. We omit the figure to illustrate client's CPU cost (Figure~\ref{proxy-cpu}) in the main text.

As shown in Figure~\ref{proxy-cpu}, when \sysname does not use proxies, the open-loop clients' CPU cost increases rapidly as the throughput grows, because each client needs to undertake heavier workload (request multicast and quorum check). The CPU intensity of clients constrains the throughput and also leads to higher latency for \sysname-Proxy (Figure~\ref{proxy-latency}). 
By contrast, after equipped with proxies, the open-loop clients' CPU cost is much lower, which enables \sysname-Proxy to outperform \sysname-Non-Proxy in both throughput and latency.

\begin{figure}[!htbp]
    \begin{minipage}{1\linewidth}
    \centering
    \subcaptionbox{Latency vs. throughput    \label{proxy-latency}}
      {
      \includegraphics[width=0.7\linewidth]{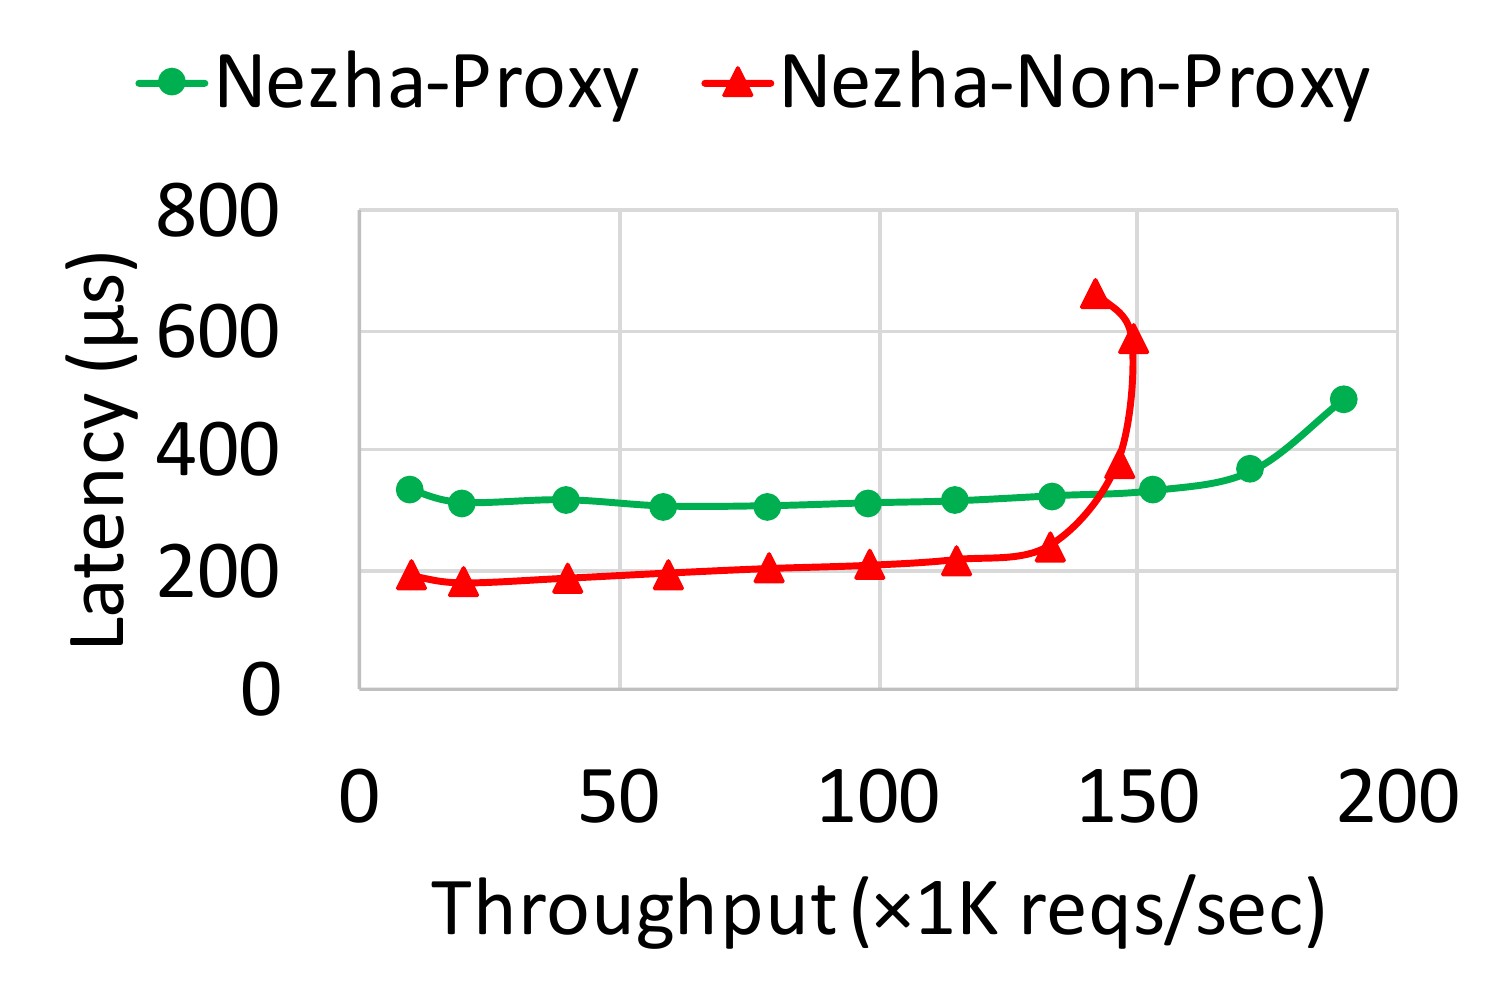}
      }
    \subcaptionbox{CPU cost vs. throughput     \label{proxy-cpu}}
      {\includegraphics[width=0.75\linewidth]{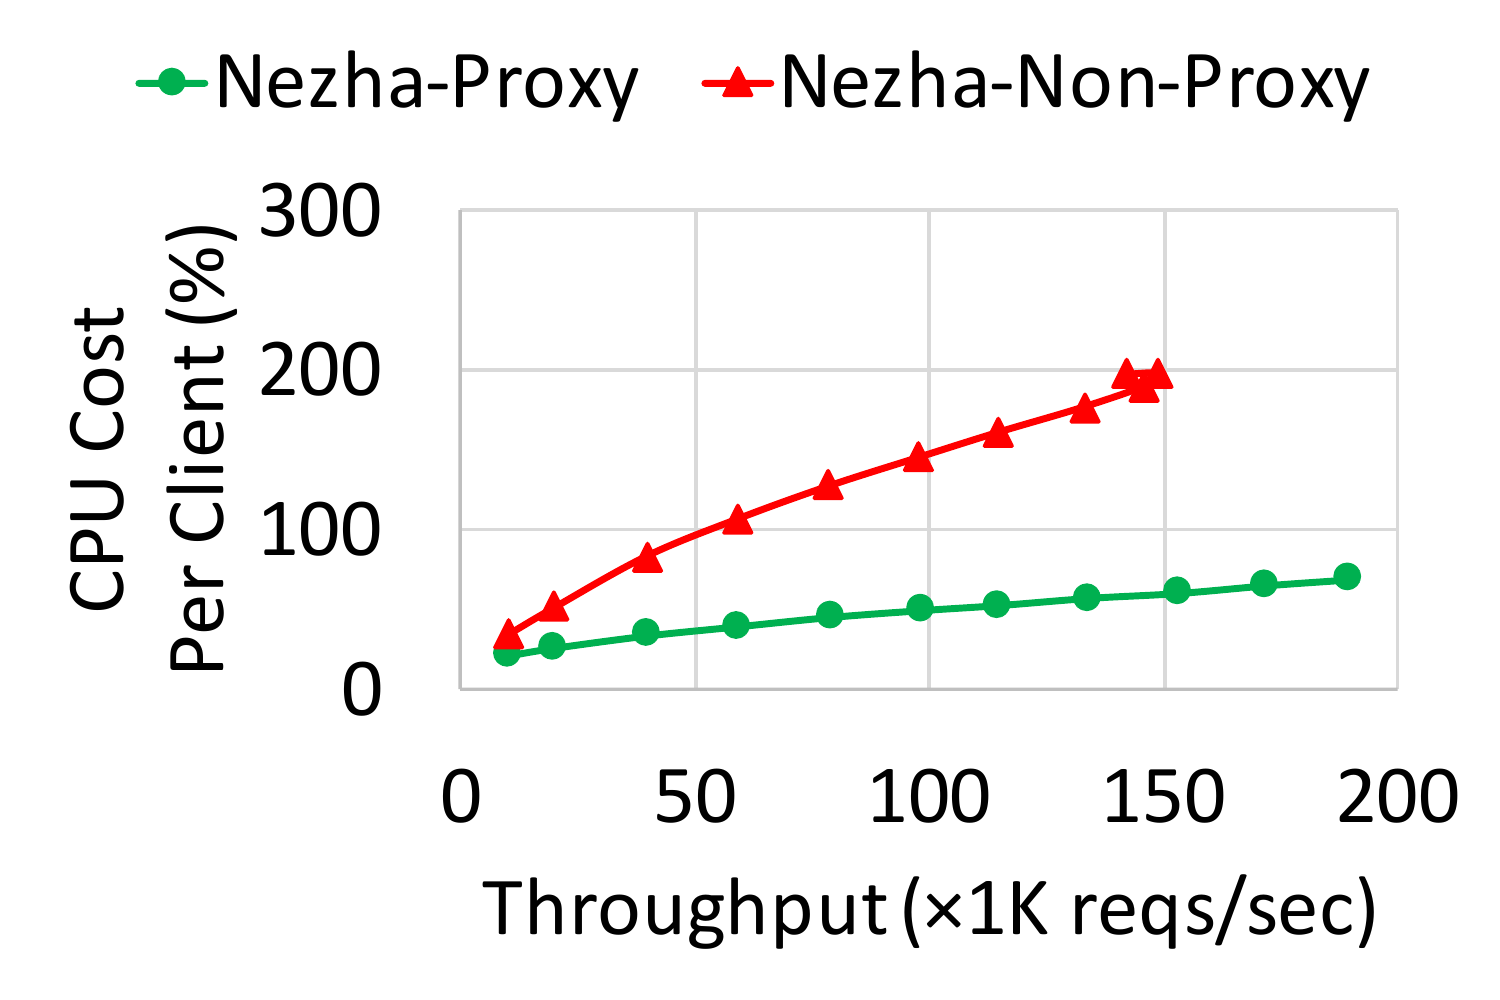}
     }
  \caption{Proxy evaluation (10 open-loop clients, 9 replicas)}
  \label{proxy-eval-supplement}
  \end{minipage}
\end{figure}
\begin{figure}[!htbp]
    \centering
    \begin{minipage}{1\linewidth}
    \centering
    \subcaptionbox{Closed-loop \label{raft-closed-loop}}
      {
      \includegraphics[width=1\linewidth]{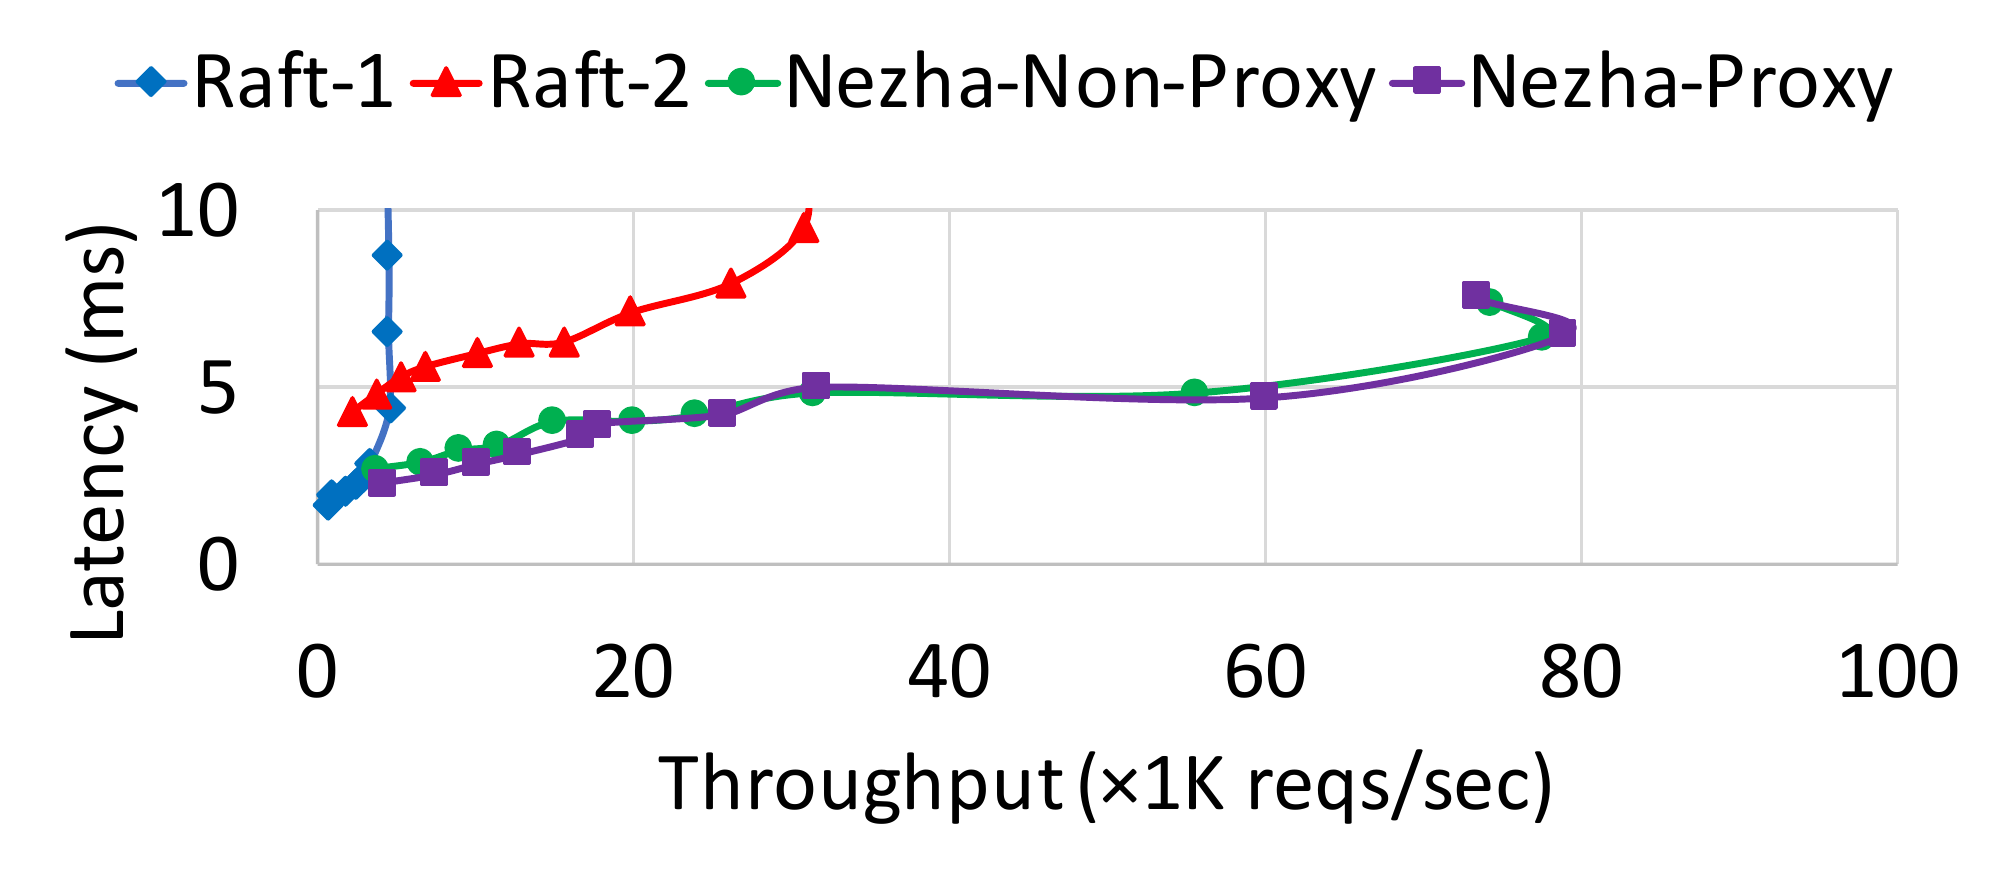}
      }
    \subcaptionbox{Open-loop \label{raft-open-loop}}
      {\includegraphics[width=1\linewidth]{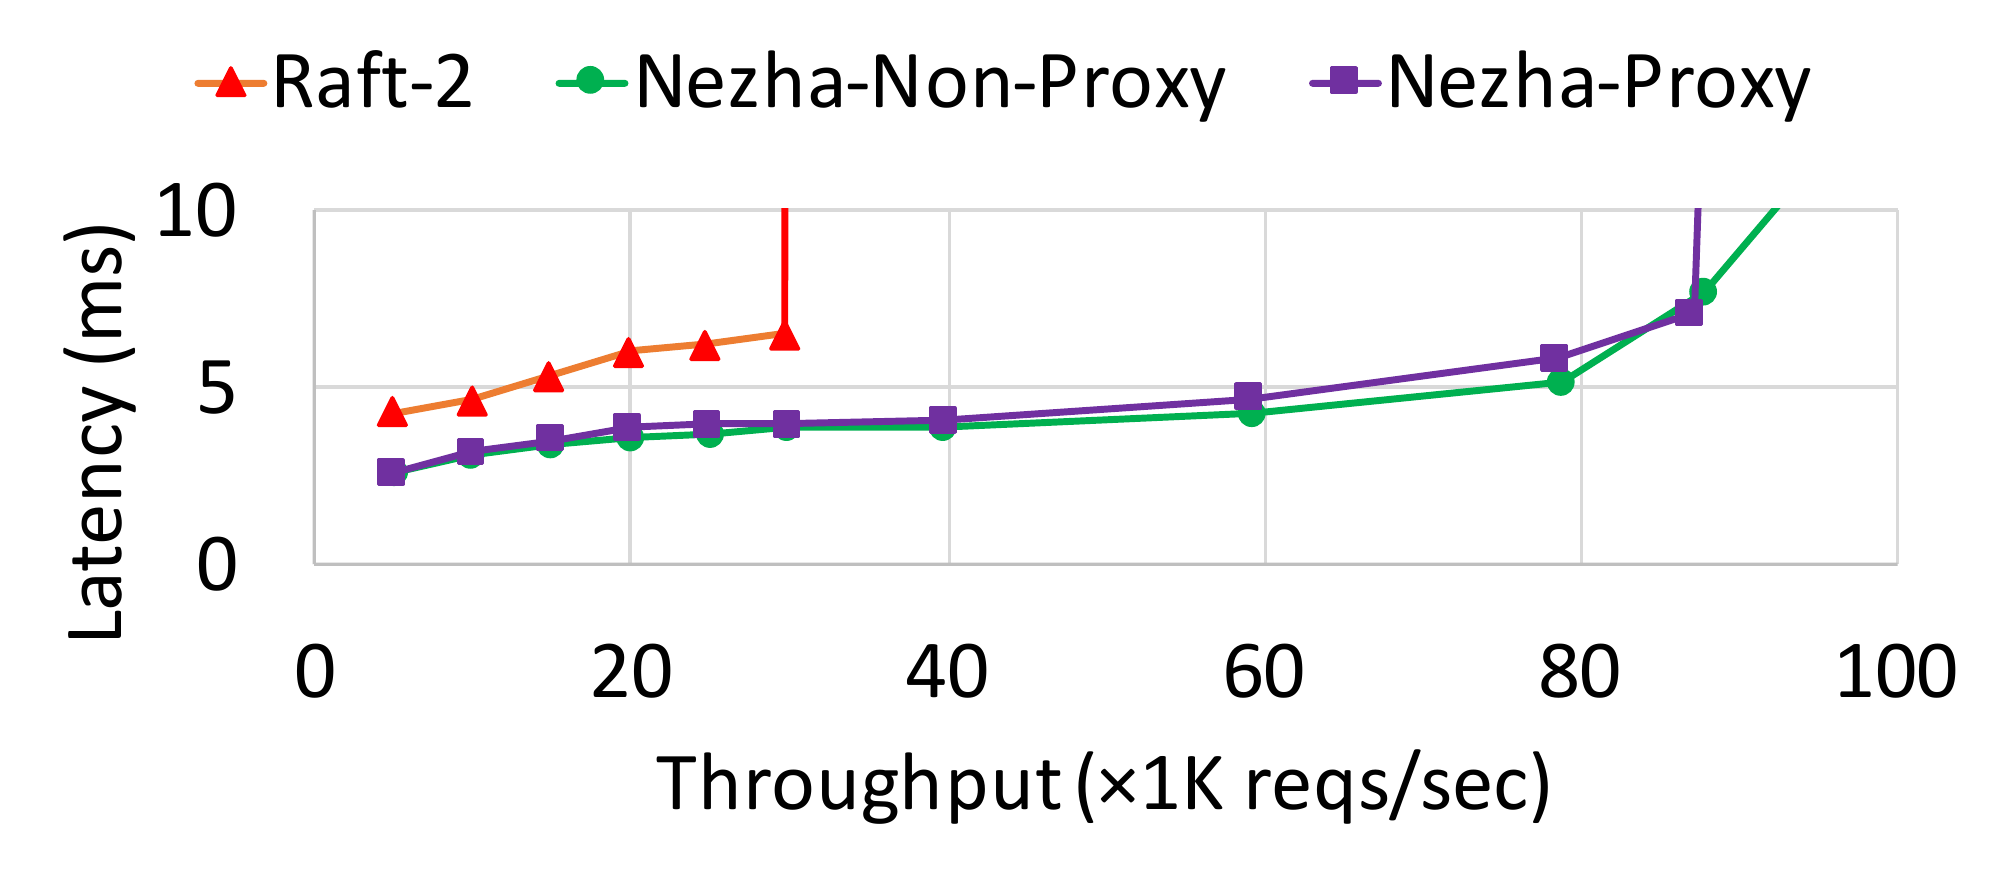}
     }
     \caption{\sysname vs. Raft}
     \label{figure-nezha-raft}
     \end{minipage}
\end{figure}

Figure~\ref{figure-nezha-raft} presents the comparison between \sysname and Raft in both closed-loop and open-loop tests. When log persistence is involved, message delays (due to network transmission) no longer dominates the latency performance. Instead, it is dominated by 
the disk write operations. Therefore, in the millisecond-level measurement of latency, \sysname-Non-Proxy and \sysname-Proxy do not show much difference. Figure~\ref{figure-nezha-raft} demonstrates that Raft is more I/O-intensive than \sysname. We omit the figure of open-loop test (Figure~\ref{raft-open-loop}) in the main text. Figure~\ref{raft-open-loop} shows that \sysname also outperforms Raft in open-loop tests.

%\sysname achieves much higher throughput than all baselines under different number of replicas. However, \sysname without proxies suffer from little degradation in closed-loop tests, because the throughput is contributed by 150 clients and each client only submits at a low rate ($\sim$1.3K reqs/sec). However, in open-loop tests with only 10 clients, the throughput of \sysname without proxies distinctly degrades from 187.8K reqs/sec to 148.7K req/sec, as the number of replicas grows. This indicates that the clients become the new bottleneck when submitting at high rates. By contrast, when equipped with proxies, neither replicas nor clients become bottlenecks, and the throughput remains high regardless of the number of replicas. We further evaluate the proxy design in \S\ref{sec:proxy}.
