# Supplementary material for: Nezha: Deployable and High-Performance Consensus Using Synchronized Clocks
Source: arXiv:2206.03285 source file (2023-03-24)
Supplement: Supplementary file 3 [file appendix.tex]

\section{Supplemental Material for \S\ref{subsec:deployment-experience}}
\setcounter{figure}{0}
\begin{figure}[H]
     \centering
     \includegraphics[width=6cm]{fig/competition/TPS.png}
     \caption{Transactions per Second vs. Day}
     \label{cs349f-tps}
\end{figure}
\begin{figure}[H]
     \centering
     \includegraphics[width=6cm]{fig/competition/OWD.png}
     \caption{Gateway to Matching Engine delay vs. Day}
     \label{cs349f-owd}
\end{figure}
\begin{figure}[H]
     \centering
     \includegraphics[width=6cm]{fig/competition/Inbound_fairness.png}
     \caption{Inbound Fairness vs. Day}
     \label{cs349f-inbound-fairness}
\end{figure}
\begin{figure}[H]
     \centering
     \includegraphics[width=6cm]{fig/competition/Outbound_Fairness.png}
     \caption{Outbound Fairness vs. Day}
     \label{cs349f-outbound-fairness}
\end{figure}
